# Supplementary material for: Dynamical Theory and Cellular Automata Simulations of Pandemic Spread: Understanding Different Temporal Patterns of Infections
Source: arXiv:2004.14787 source file (2020-04-30)
Supplement: Supplementary file 1 [file SI.pdf]

# Dynamical Theory and Cellular Automata Simulations of Pandemic Spread: Understanding Different Temporal Patterns of Infections


Saumyak Mukherjee, Sayantan Mondal and Biman Bagchi*

Solid State and Structural Chemistry Unit
Indian Institute of Science, Bengaluru – 560012, India
*Email: bbagchi@iisc.ac.in


Here, we present the temporal evolution of the four sections of the society, namely susceptibles (S), infectives (I), cured (C) and dead (D), as obtained from stochastic cellular automata simulations. The temporal patterns are studied by varying different parameters in the simulation.

## SI. Temporal Profiles of Population as a Function of Initial Fraction of Susceptibles and Infectives

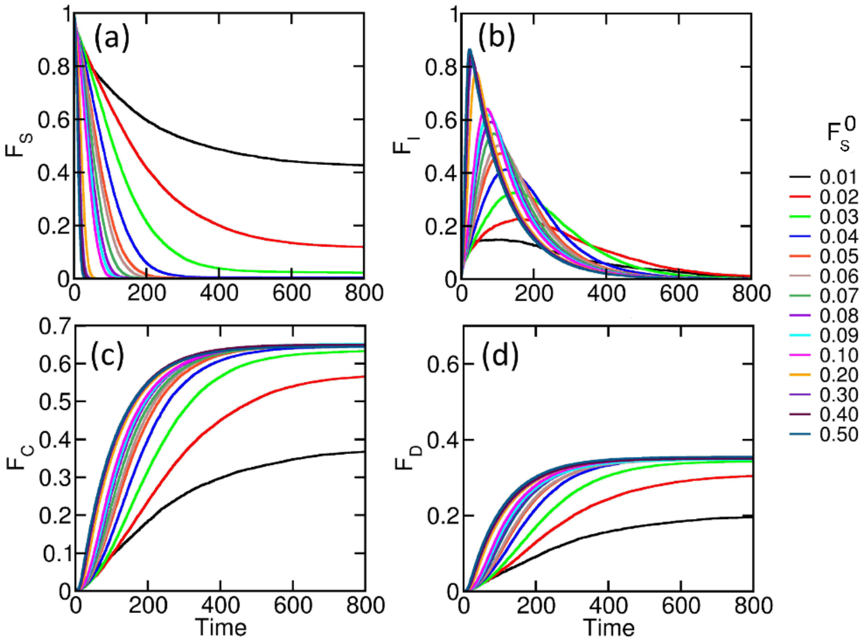


**Figure S1.** Variation of the fraction of (a) susceptibles ($F_S$), (b) infected ($F_I$), (c) cured ($F_C$), and (d) dead ($F_D$) with respect to changing fraction of healthy population when the fraction of initially infected population ( $F_I^0 = 0.001$ ) remains fixed. In all these simulations 70% young population is considered with a cut-off age of 50 years.

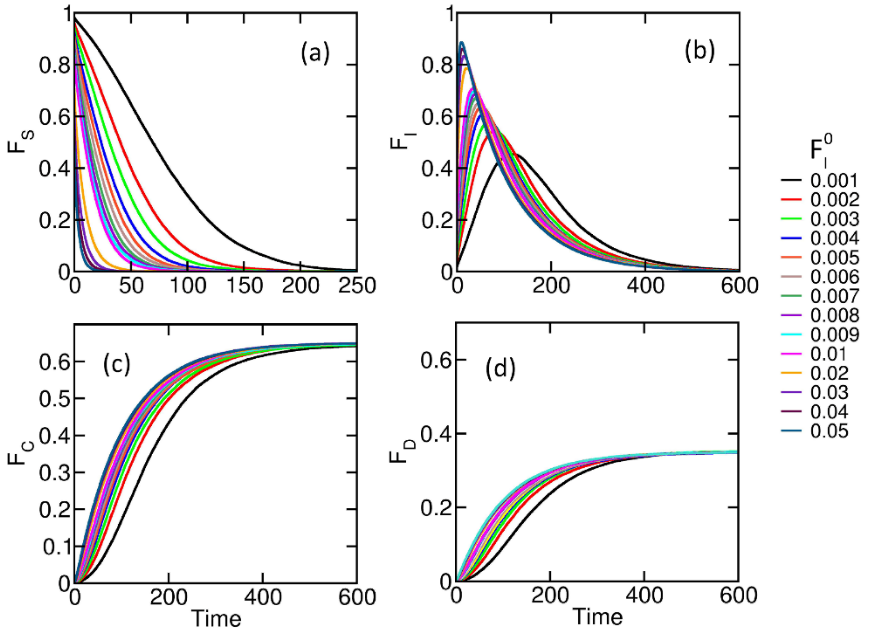


**Figure S2.** Variation of (a) $F_S$, (b) $F_I$, (c) $F_C$, and (d) $F_D$ with time for different fraction of initially infected population ($F_I^0$) while the fraction of initially infected population remains fixed ($F_I^0$ =0.001).

## SII. Temporal Profiles of Population as a Function of the Fraction of Young Population

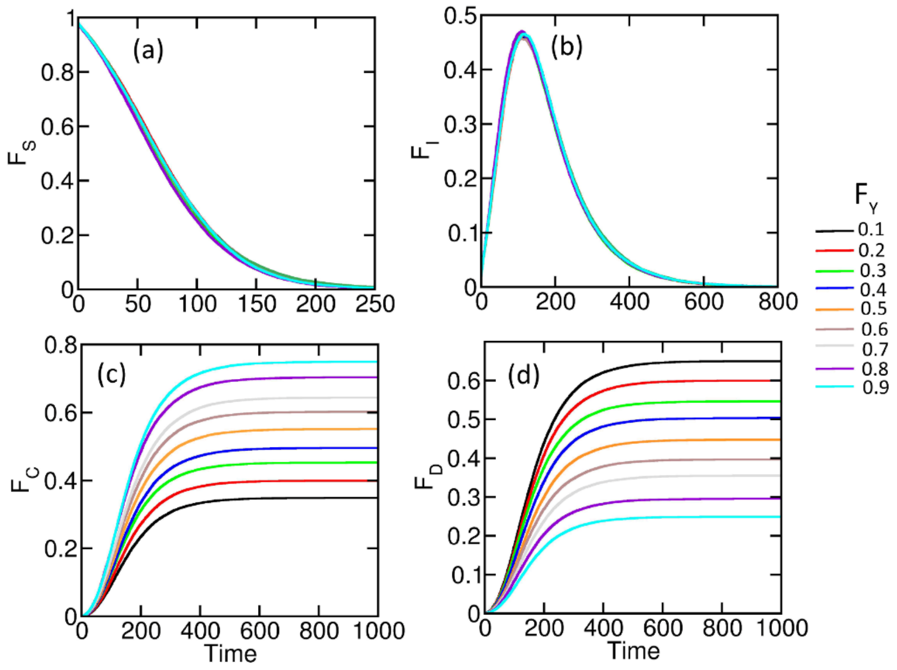

**Figure S3.** Variation in the fraction of (a) susceptibles (S), (b) infected (I), (c) cured (C), and (d) dead (D) population against time for different fraction of younger population ($F_Y$). The patterns of $F_S$ and $F_I$ shows no change as the probability of transmission remains the same for the older and younger people. However there is a drastic change in the number of cured and dead patients.

## SIV. Temporal Profiles of Population as a Function of the Time Period of Infection

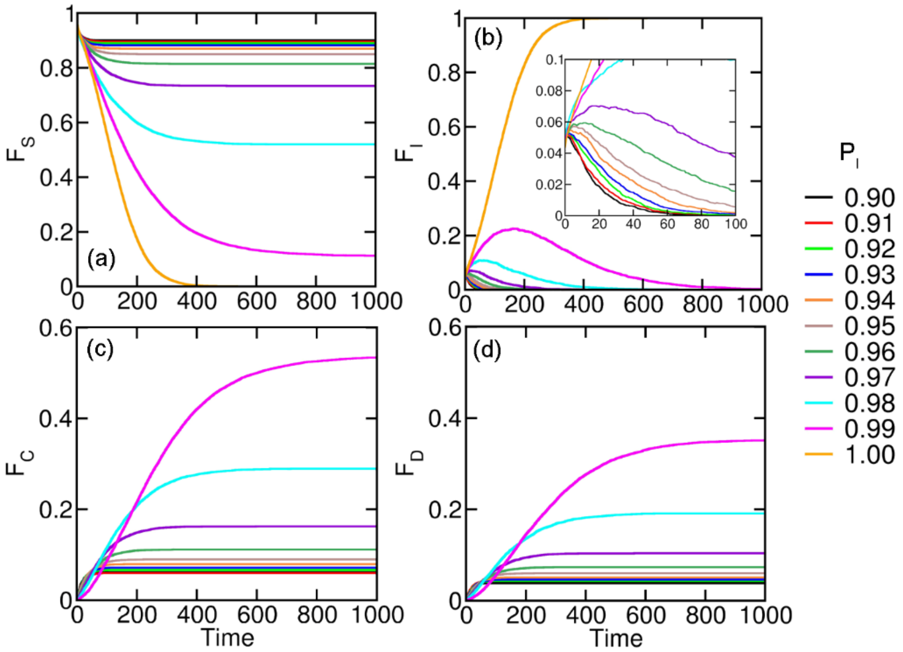


**Figure S4.** The time evolutions of the different categories of the total population as a function of $P_I$. (a) Susceptibles, (b) Infectives, (c) Cured/recovered, and (d) Dead. The values of $P_I$ are colour coded as mentioned on the right hand side of the figure. For these simulations, $P_{R_Y}$ = 0.8, $P_{R_O}$ = 0.3 and $A$ = 50.

## SV. Temporal Profiles of Population as a Function of Quarantine and Social Distancing

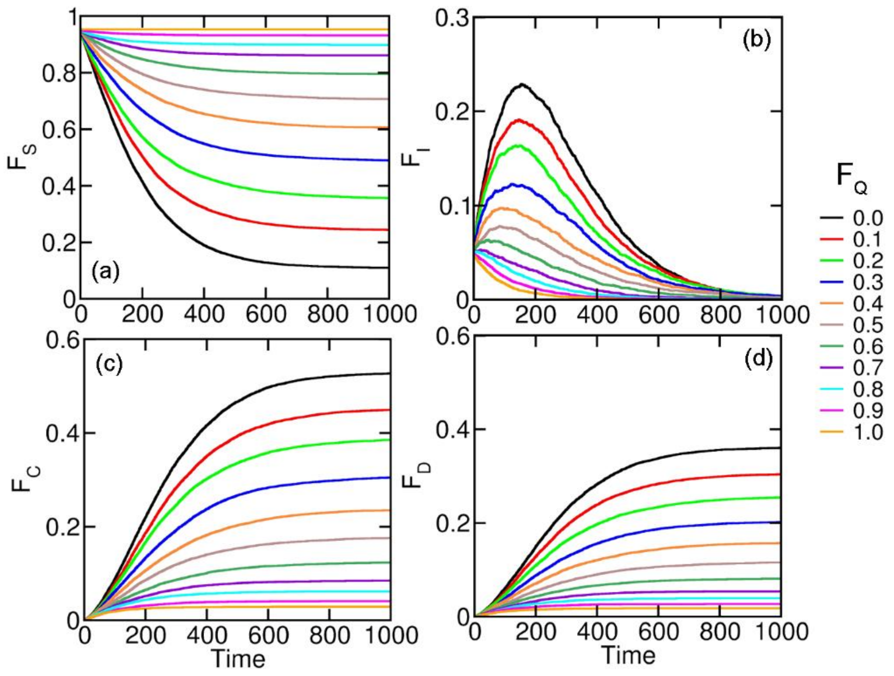


**Figure S5.** Time progression of the four sections of the population with varying values of the fraction of people abiding by quarantine and lock down norms. (a) Susceptible, (b) Infected, (c) Cured, and (d) Recovered. Extensive quarantine translates to greater chance of survival.

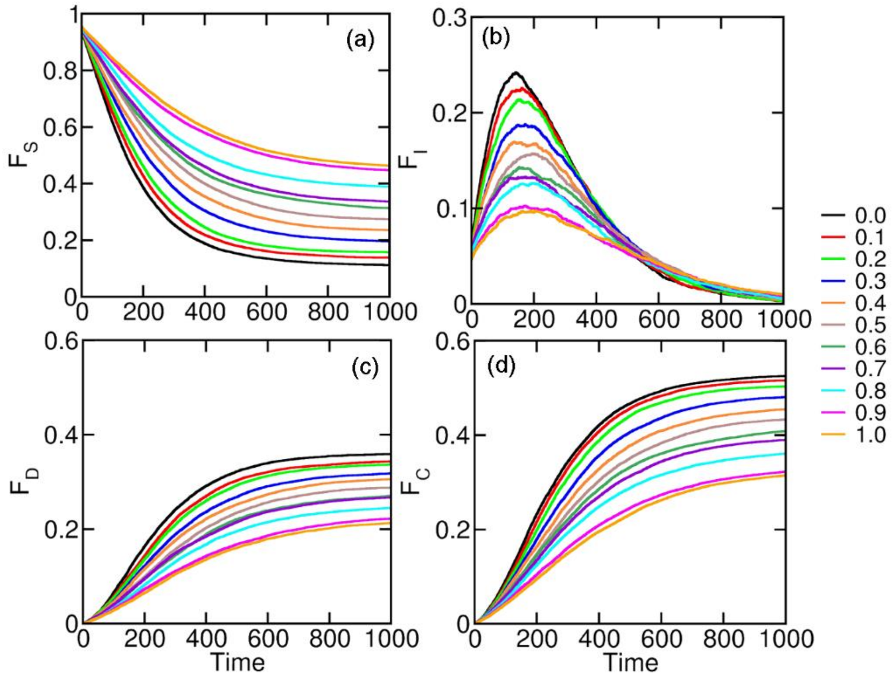


**Figure S6.** Time progression of the four sections of the population with varying values of the fraction of people maintaining social distancing. (a) Susceptible, (b) Infected, (c) Cured, and (d) Recovered. The effect of social distancing is much less than home quarantine.
